# Supplementary material for: Identifying the fingerprints of topological states by tuning magnetoresistance in a semimetal: the case of topological half-Heusler Pt1-xAuxLuSb
Source: arXiv:2012.12633 ancillary file (2022-01-04)
Supplement: Supplementary file 1 [file SupplementaryInformation.pdf]

# Revealing quantum Hall states in epitaxial topological half-Heusler semimetal

Shouvik Chatterjee,[1,2,*] Felipe Crasto de Lima,[3,4] John A. Logan,[5] Yuan Fang,[6] Hadass Inbar,[5] Aranya Goswami,[1] Connor Dempsey,[1] Shoaib Khalid,[7,3] Tobias Brown-Heft,[5] Yu-Hao Chang,[5] Daniel Pennacchio,[5] Nathaniel Wilson,[5] Jason Dong,[5] Shalinee Chikara,[8] Alexey Suslov,[8] Alexei V. Fedorov,[9] Dan Read,[10] Jennifer Cano,[6,11] Anderson Janotti,[3] and Christopher J. Palmstrøm[1,5,*]

*[1]Department of Electrical and Computer Engineering, University of California, Santa Barbara, CA 93106, USA*
*[2]Department of Condensed Matter Physics and Materials Science, Tata Institute of Fundamental Research, Homi Bhabha Road, Mumbai 400005, India*
*[3]Department of Materials Science and Engineering, University of Delaware, Newark, DE 19716, USA*
*[4]Instituto de Física, Universidade Federal de Uberlândia, C.P. 593, 38400-592, Uberlândia, MG, Brazil*
*[5]Materials Department, University of California, Santa Barbara, CA 93106, USA*
*[6]Department of Physics and Astronomy, Stony Brook University, Stony Brook, New York, 11974, USA*
*[7]Department of Physics and Astronomy, University of Delaware, Newark, DE 19716, USA*
*[8]National High Magnetic Field Laboratory, Tallahassee, FL 32310, USA*
*[9]Advanced Light Source, Lawrence Berkeley National Laboratory, Berkeley, CA 94720, USA*
*[10]School of Physics and Astronomy, Cardiff University, Cardiff CF24 3AA, UK*
*[11]Center for Computational Quantum Physics, Flatiron Institute, New York, New York, 10010, USA*

## I. SAMPLE GROWTH AND CHARACTERIZATION

$Pt_{1-x}Au_xLuSb$ thin films are grown on InSb buffer layers synthesised on unintentionally doped GaAs (001) substrates. Thin films are single phase with [001] out-of-plane orientation and remains pseudomorphic across the whole doping range from x=0 to x=1/2 in $Pt_{1-x}Au_xLuSb$, as shown in Fig. S1a,b. Gold (Au) has a larger atomic radius compared to platinum (Pt), hence naively a larger lattice constant is expected for substitutionally alloyed films. This is also supported by DFT calculations that predict an equilibrium lattice constant of 6.77 Å for AuLuSb, greater than what is theoretically estimated for PtLuSb (6.54 Å). Experimentally, PtLuSb lattice constant is found to be 6.457 Å (see Fig. S1a,b.)[1,2], which is close to the InSb lattice constant of 6.479 Å. For $Pt_{1-x}Au_xLuSb$ thin films, contrary to expectation, the out-of-plane lattice constant is found to decrease with increasing Au content that starts to saturate at higher Au concentrations. Estimated out-of-plane lattice parameter as a function of Au concentration from x-ray diffraction measurements is shown in Fig. S1c. Enhanced Au-Au bonding strength with a strong propensity to form Au dimer bonds, as has been recently predicted and observed in Au based heaxgonal half-Heusler compounds[3,4], might be responsible for the observed anomalous behavior in the cubic half-Heusler structures realized in the present study. High-angle annular dark field scanning transmission electron microscopy (HAADF-STEM) image shown in Fig S1d. reveals a continuous Sb sub-lattice that extends from the InSb buffer layer to the $Pt_{1-x}Au_xLuSb$ thin films confirming excellent film quality and negligible inter-diffusion at the interface. Furthermore, sharp, streaky RHEED pattern, shown in Fig. S2 and scanning tunnelling microscopy images, shown in Fig. S3 confirms smooth morphology of the film surface. In Fig. S4 we characterise the transport properties of the 270 nm thick InSb buffer layer used to synthesize $Pt_{1-x}Au_xLuSb$ thin films. InSb being a narrow band-gap semiconductor is a source of parallel conduction channel in our Hall bar devices, which contributes to a finite conductance leading to the longitudinal magnetoresistance not touching zero and the quantum Hall plateaus not quantized to the values of $\nu\frac{e^2}{h}$, where $\nu$ is either an integer or a half-integer. However, the InSb buffer layer shows trivial magnetotransport behavior with the longitudinal magnetoresistance showing a saturating behavior of only 6% at 45 Tesla and the Hall effect exhibiting a linear electron-like behavior at high fields. This is very different from the magntotransport properties of $Pt_{1-x}Au_xLuSb$ thin films described in the main text (Figs. 1,2, and 4). We can therefore confidently establish that the observed transport properties including the linear magnetoresistance behavior and quantum Hall effect is entirely due to $Pt_{1-x}Au_xLuSb$. We note that the same InSb buffer layer, magnetotransport properties of which is shown in Fig. S4, is used to synthesize all the $Pt_{1-x}Au_xLuSb$ thin films that are used for magnetotransport measurements in the present study.

*Authors to whom correspondence should be addressed: `shouvik.chatterjee@tifr.res.in,cjpalm@ucsb.edu`

## II. BAND INVERSION IN $Pt_{1-x}Au_xLuSb$ AND ESTIMATION OF BAND BENDING

The topological character of $Pt_{1-x}Au_xLuSb$ is preserved by going from x=0.0 to x=0.5. That is, the energy ordering of the $s$ and $p$ orbital character in the bulk $\Gamma_8$ and $\Gamma_6$ bands remains inverted even after replacing 50% of the platinum (Pt) atoms with gold (Au) in $Pt_{1/2}Au_{1/2}LuSb$, as shown in Fig. S5. Due to extra electrons added by Au atoms in the $Pt_{1-x}Au_xLuSb$, there is an upward shift of the Fermi level (in relation to $\Gamma_8$) for the alloyed case (Fig. S5b).

The change in carrier concentration and the Fermi wave vector ($k_F$) as a function of the position of the chemical potential, as estimated from a bulk DFT calculation of PtLuSb, is shown in Fig. S6. The zero of the chemical potential is at the bulk $\Gamma_8$ point. We have utilized the dependence of carrier concentration on the position of the chemical potential (Fig. S6) and the carrier concentration estimated from the Hall coefficient (Fig. 1b,c in the main text) to estimate the position of the bulk Fermi level with respect to the $\Gamma_8$ point ($\Delta_1$) in $Pt_{1-x}Au_xLuSb$ thin films, shown in Fig. 1d in the main text. Topological surface state (TSS) in $Pt_{1-x}Au_xLuSb$ thin films exhibits linear dispersion at binding energies away from the Dirac point as shown by the ARPES measurements. Linear fits to the TSS observed in the ARPES data, as shown in Fig. 2 in the main text, is used to estimate linear extrapolated crossing point (LECP) and the position of the surface Fermi level with respect to LECP ($\Delta_3$) in $Pt_{1-x}Au_xLuSb$ thin films. The position of LECP with respect to the $\Gamma_8$ point ($\Delta_2$) in $Pt_{1-x}Au_xLuSb$ is estimated from corresponding DFT slab calculations as shown in Fig. S7. Finally, the band bending, $\Delta_{bb}$ can be estimated as

$$\Delta_{bb} = \Delta_1 + \Delta_2 + \Delta_3 \tag{S1}$$

as shown in the schematic in Fig. 2j in the main text. We note that in our calculations LECP does not correspond to the calculated Dirac points (Fig. S7) due to a change in dispersion of the TSS very close to the Dirac point, which is not observed in the ARPES measurements (Fig. 2 in the main text). We utilize estimated LECP instead of corresponding Dirac points to estimate $\Delta_2$ in order to maintain consistency between theory and experiment, where a similar linear extrapolation is used to estimate $\Delta_3$ from the ARPES data, and together we get a correct and internally consistent estimate for $\Delta_2 + \Delta_3$, which is the relevant quantity for estimation of band bending. Individual values of $\Delta_1$, $\Delta_2$, $\Delta_3$, and $\Delta_{bb}$ are shown in Table S1, where a positive value for $\Delta_{bb}$ indicates an upward band bending.

## III. ANISOTROPIC G-FACTOR

The g-factor in the *two Dirac model*, described in the main text, is the effective g-factor that takes into account orbital contributions of the adjacent bulk bands. The band structure of the $\Gamma_8$ manifold, which constitutes the bulk bands near the Fermi level in $Pt_{1-x}Au_xLuSb$ is anisotropic, as shown in Fig S5(c), and hence, it is expected that the g-factor in $Pt_{1-x}Au_xLuSb$ would also be anisotropic. We track the Zeeman-split minima in magnetoresistance corresponding to the n=2 quantum Hall state in $Pt_{7/8}Au_{1/8}LuSb$ and $Pt_{5/8}Au_{3/8}LuSb$ as the magnetic field vector is rotated from [001] to [110] through [111], shown in Fig. S9 and Fig. S10, respectively. The effective g-factor and Fermi level ($E_F$) is extracted from the positions of the magnetoresistance minima using Eqn. 6 in the main text noting that the orbital component is dependent only on the perpendicular component of the magnetic field vector ($\mu_0$Hcos($\theta$)), whereas the Zeeman component depends on the magnitude of the applied field ($\mu_0$H). We keep $\Delta_h$ (half of the hybridization gap) and $\Delta_i$ (inversion symmetry breaking) fixed to the value obtained from fits to the whole magnetoresistance spectrum under perpendicular magnetic field ($\theta = 0$), shown in Table 1 of the main text. The estimated g-factor has a minima between 40 and 50 degrees, when the magnetic field vector points at a direction close to [111] crystallographic axis for both $Pt_{7/8}Au_{1/8}LuSb$ and $Pt_{5/8}Au_{3/8}LuSb$.

## IV. WEAK ANTI-LOCALIZATION IN $Pt_{1-x}Au_xLuSb$ THIN FILMS

Observation of two-dimensional weak anti-localization (WAL) behavior, shown in Fig. S11 in $Pt_{1-x}Au_xLuSb$ thin films, is further indicative of the presence of strongly spin-orbit coupled topological surface states (TSS) from where an estimate of the surface-bulk coupling can be obtained. WAL behavior in $Pt_{1-x}Au_xLuSb$ can be well fitted with the Hikami-Larkin-Nagaoka(HLN) theory[5] given by

$$\Delta G = -\alpha \frac{e^2}{\pi h}[\Psi(\frac{1}{2} + \frac{B_\phi}{B_\perp}) - ln(\frac{B_\phi}{B_\perp})] \tag{S2}$$

where $\Psi$ is the digamma function, and $B_\phi = \frac{\hbar}{4el_\phi^2}$ is the characteristic magnetic field corresponding to the phase coherence length $l_\phi$. The pre-factor $\alpha$ captures the surface-bulk coupling[6]. The magnitude of $\alpha$ is equal to $\frac{1}{2}$ for

an independent strongly spin-orbit coupled two-dimensional channel, which is reduced with enhanced surface-bulk coupling. A lower value of $\alpha$ for $Pt_{7/8}Au_{1/8}LuSb$ compared to $Pt_{5/8}Au_{3/8}LuSb$, shown in Fig. S11e, indicates higher surface-bulk coupling in the low Au doped sample, in agreement with the magnetotransport data at high magnetic fields, shown in Fig. 3 in the main text. The phase coherence length ($l_\phi$) is found to be similar in both the samples, with a slightly larger values of $l_\phi$ in $Pt_{5/8}Au_{3/8}LuSb$ at lower temperatures, again indicative of lower surface-bulk coupling in the higher gold doped samples. Temperature dependence of the phase coherence length shows a power-law behavior $l_\phi \propto T^{-0.54}$, indicative of Nyquist dephasing due to electron-electron interaction effects in two-dimensional systems[7]. However, at low temperatures we find evidence for an enhanced dephasing rate, which could be due to the coupling between the surface states and quasi-localised bulk carriers in the variable-range hopping (VRH) regime, as has been observed in other three-dimensional topological insulators[8].

## V. ADDITIONAL DATA FOR $Pt_{3/4}Au_{1/4}LuSb$ AND $Pt_{1/2}Au_{1/2}LuSb$

Similar magnetotransport properties, as has been shown in Fig. 3 in the main text, is observed in $Pt_{1-x}Au_xLuSb$ thin films for other Au concentrations such as $Pt_{3/4}Au_{1/4}LuSb$ and $Pt_{1/2}Au_{1/2}LuSb$. The data for these samples are shown in Fig. S12. Note that linear magnetoresistance behavior is observed in $Pt_{3/4}Au_{1/4}LuSb$ up to a magnetic field of $\approx$ 15 Tesla. The linear magnetoresistance behavior is observed up to 22 Tesla for $Pt_{7/8}Au_{1/8}LuSb$ (Fig. 3 in the main text). Thus, with the increase in Au concentration and at higher magnetic fields the linear magnetoresistance gradually transmutes into a quantum hall phase with well-defined minima in magnetoresistance and corresponding quantum Hall plateaus in $Pt_{1-x}Au_xLuSb$ thin films. The same *two-Dirac model*, described in the main text, can be used to understand the quantum Hall phase in $Pt_{3/4}Au_{1/4}LuSb$ and $Pt_{1/2}Au_{1/2}LuSb$, shown in Fig. S13. The model parameters are shown in Table S2.

## VI. *K.P* MODEL

The electronic states near the bulk $\Gamma$ point for the half-Heusler compound PtLuSb arise from the $j = 3/2$ $\Gamma_8$ representation, primarily consisting of spin-orbit coupled Sb $p$-orbitals. The dispersion of the $\Gamma_8$ bands can be modelled using $k.p$ theory, where upto a quadratic order in $k$ the Hamiltonian consists of the Luttinger-Kohn model[9] and a linear inversion breaking term[10], which can be written as

$$H_0 = \alpha k^2 + \beta\Sigma_i k_i^2 J_i^2 + \gamma\Sigma_{i\neq j} k_i k_j J_i J_j + \delta\Sigma_i k_i (J_{i+1} J_i J_{i+1} - J_{i+2} J_i J_{i+2}) \tag{S3}$$

where $i$ goes over $x, y, z$ and $J_{x,y,z}$ are the 4×4 matrices that represent $j = 3/2$ angular momentum operators satisfying the commutation relations $[J_i, J_{i+1}] = \iota J_{i+2}$. The parameters in the model ($\alpha$, $\beta$, $\gamma$, and $\delta$) are estimated by simultaneously fitting the model to the calculated band structure of PtLuSb from density functional theory (DFT) along [100] and [110], as shown in Fig. S14. From the $k.p$ theory, the effective mass along [100] is given by

$$m^* = \frac{\hbar^2}{2(\alpha + \frac{5}{4}\beta \pm \beta)} \tag{S4}$$

which is estimated to be $0.18m_e$ (upward dispersive branch) and $-0.17m_e$ (downward dispersive branch). Within a simple one-dimensional confinement model (confinement is along the film growth direction in our case), the discrete energy levels are given by

$$E_n = \frac{n^2\pi^2\hbar^2}{2m^*t^2} \tag{S5}$$

where $n$ is a non-zero integer, $m^*$ is the effective mass, and $t$ is the film thickness. For a 15 nm thick film, the confinement induced band gap is estimated to be $\Delta = 18.72$ meV.

The $k.p$ model, described above is used to calculate the bulk Landau levels under a quantizing magnetic field. The Zeeman effect is taken into account in these calculations by incorporating plausible g-factor values, results for which are shown in Fig. S15.

In a magnetic field $B$, we add the Zeeman term:

$$H_Z = g\mu \mathbf{J} \cdot \mathbf{B}. \tag{S6}$$

To be concrete, we take the following matrix form for $\mathbf{J} = (J_x, J_y, J_z)$, which are the spin-3/2 matrices:

$$J_x = \begin{pmatrix} 0 & \frac{\sqrt{3}}{2} & 0 & 0 \\ \frac{\sqrt{3}}{2} & 0 & 1 & 0 \\ 0 & 1 & 0 & \frac{\sqrt{3}}{2} \\ 0 & 0 & \frac{\sqrt{3}}{2} & 0 \end{pmatrix}, \qquad J_y = \begin{pmatrix} 0 & -i\frac{\sqrt{3}}{2} & 0 & 0 \\ i\frac{\sqrt{3}}{2} & 0 & -i & 0 \\ 0 & i & 0 & -i\frac{\sqrt{3}}{2} \\ 0 & 0 & i\frac{\sqrt{3}}{2} & 0 \end{pmatrix}, \qquad J_z = \begin{pmatrix} \frac{3}{2} & 0 & 0 & 0 \\ 0 & \frac{1}{2} & 0 & 0 \\ 0 & 0 & -\frac{1}{2} & 0 \\ 0 & 0 & 0 & -\frac{3}{2} \end{pmatrix} \tag{S7}$$

To derive the Landau level spectrum for a static magnetic field $B$ in the $z$ direction, we make the canonical substitutions: $k_{x,y} \longrightarrow \Pi_{x,y} \equiv k_{x,y} + eA_{x,y}/\hbar$, where $[\Pi_x, \Pi_y] = ieB$. We can then define the raising and lowering operators:

$$a = \frac{1}{\sqrt{2eB\hbar}}\left(\Pi_x - i\Pi_y\right), \qquad a^\dagger = \frac{1}{\sqrt{2eB\hbar}}\left(\Pi_x + i\Pi_y\right), \tag{S8}$$

which obey $[a, a^\dagger] = 1$.

In terms of the raising and lowering operators, the Hamiltonian $H_0 + H_Z$ takes the form:

$$\begin{aligned} H = &-E_F + \left[2\alpha B\left(a^\dagger a + \frac{1}{2}\right) + \alpha k_z^2\right] \\ &+ \beta\left[\frac{Be\hbar}{4}\left(\left(a^2 + \left(a^\dagger\right)^2\right)(J_+^2 + J_-^2) + \left(a^\dagger a + \frac{1}{2}\right)\left(\frac{15}{2} - 2J_z^2\right)\right) + k_z^2 J_z^2\right] \\ &+ \gamma\left[\frac{Be\hbar}{4}\left(a^2 - \left(a^\dagger\right)^2\right)(J_+^2 - J_-^2) + \sqrt{\frac{Be\hbar}{2}}k_z\left(a\left(J_+J_z + J_zJ_+\right) + a^\dagger\left(J_-J_z + J_zJ_-\right)\right)\right] \\ &+ \delta\left[\sqrt{\frac{Be\hbar}{2}}\left(aU + a^\dagger U^\dagger\right) + k_z(J_xJ_zJ_x - J_yJ_zJ_y)\right] \\ &+ g\mu_B B J_z/\hbar, \end{aligned} \tag{S9}$$

where

$$U = J_yJ_xJ_y - J_zJ_xJ_z + iJ_zJ_yJ_z - iJ_xJ_yJ_x, \tag{S10}$$

and $J_\pm = J_x \pm iJ_y$.

To solve this Hamiltonian, we work in the Fock basis

$$\psi = \begin{pmatrix} \sum_{n=0}^N C_{n,1}|n\rangle \\ \sum_{n=0}^N C_{n,2}|n\rangle \\ \sum_{n=0}^N C_{n,3}|n\rangle \\ \sum_{n=0}^N C_{n,4}|n\rangle \end{pmatrix} \tag{S11}$$

with $N \longrightarrow \infty$. For a numerical calculation, we must truncate the Fock basis at some finite $N$.

The matrix representation of $H_0 + H_Z$ is then a sparse $4N$ by $4N$ matrix, whose eigenvalues give the Landau level spectrum.

In a thin film, $k_z = \frac{n\pi}{La}$ takes on discrete values, where $n$ = 0,1,2,...,$L$-1, where $L$ is the number of layers, and $a$ is the lattice constant. In our case, the film thickness of PtLuSb corresponds to $L \approx 23$ layers. We expect to obtain a set of Landau levels corresponding to each such discrete $k_z$ value. However, for the range of magnetic field in our experiment, we need to consider only $k_z = 0$, because the spectrum is gapped at larger $k_z$.

The chemical potential for $Pt_{1/2}Au_{1/2}LuSb$, $Pt_{5/8}Au_{3/8}LuSb$, $Pt_{3/4}Au_{1/4}LuSb$, and $Pt_{7/8}Au_{1/8}LuSb$ are 2.025, 1.75, 1.375, and 0.775 meV, respectively, as shown in Fig. 1d in the main text. We set the truncation number in Eq. (S11) to $N = 100$. The $g$-factor is taken to be 10 $\mu_B/\hbar$.

The Landau fan diagram $E$ vs $1/B$ for the fit is shown in Fig. S15**a**. From the plot, we see that for the set of parameters, the Landau levels cross the Fermi energy at fields $B < 3.3$ T and the bulk quantum limit is achieved for $B \approx 3.3T$. However, in the experiment, we see the Landau levels at a much larger magnetic field, $B > 10$ T. For larger $g$, the bulk quantum limit is achieved at even smaller values of $B$, thereby making the difference between the experimentally observed Hall conductance plateaus and the theoretically computed Hall conductance plateaus from the bulk Landau levels even larger.

We also compute the Landau levels with $g = 0$, as shown in Fig. S15**b**. The bulk quantum limit is now achieved at $B = 8.97$ T, which is still much smaller than the field values at which quantum Hall plateaus have been observed in the experiment. It is interesting to note that signatures of the quantum Hall phase in $Pt_{1-x}Au_xLuSb$ thin films only become manifest for approximately $B > 10$ T, when the samples are in the bulk quantum limit. Therefore, we conclude that the Hall conductance plateaus observed in the magnetotransport data do not originate from the bulk bands.

## VII. QUANTUM HALL FROM MAGNETIC FIELD INDUCED WEYL FERMI ARCS

In $Pt_{1-x}Au_xLuSb$ Weyl points can appear under the application of magnetic field due to the Zeeman effect from the symmetry protected crossings between $J_z = 1/2$ and $J_z = 3/2$ and between $J_z = -1/2$ and $J_z = 3/2$ bands.[11] We only consider those Weyl points that can result in a non-zero Fermi arc length on the (001) surface because only these Fermi arcs can lead to a possible appearance of quantum oscillations in our transport measurements where the magnetic field vector **B** is parallel to the [001] crystallographic direction. An example of such Weyl points arising from a protected crossing of the $J_z = -1/2$ and $J_z = 3/2$ bands is shown in Fig. S16.

We consider a pair of Weyl points at $\pm\mathbf{k_w}$, where the Fermi velocity is given by

$$v_w = \frac{|\mathbf{k_w}|}{m^*} \tag{S12}$$

$m^*$ being the effective mass. In our case $|\mathbf{k_w}|$ is a monotonically increasing function of the magnetic field B

$$|\mathbf{k_w}| = Af(B) \tag{S13}$$

where A is a constant. Utilizing 'energy-time' quantization condition within a semiclassical formalism, as has been described in Ref.[12] we obtain

$$E_n = \frac{\pi v_w(n+\gamma)}{t + k_0/eB} \tag{S14}$$

where $t$ is the film thickness, $\gamma$ is a constant of order unity encoding low-$n$ quantum effects (see Ref.[12]), $k_0$ is the Fermi arc length, and $n$ is the Landau level index. In the simplest case, when the Fermi arc is a straight line, $k_0 = 2|\mathbf{k_w}|$. Without loss of generality we can assume $k_0 = c|\mathbf{k_w}|$, where $c \geq 2$. For a constant chemical potential $\mu$ and varying magnetic field as is the case for magnetotransport measurements Eqn. S14 can be written as

$$\mu = \frac{\pi v_w(n+\gamma)}{t + k_0/eB_n} = \frac{\pi \frac{Af(B_n)}{m^*}(n+\gamma)}{t + \frac{cAf(B_n)}{eB_n}} \tag{S15}$$

where $B_n$ is the magnetic field at which $n^{th}$ Landau level is crossed. Therefore,

$$n = \frac{m^*\mu}{\pi A}[\frac{t}{f(B_n)} + \frac{cA}{eB_n}] \tag{S16}$$

From Eqn. S15 we can infer that the distance between the adjacent Landau levels in magnetic field is a monotonically decreasing function of Landau level indices, similar to the Landau levels obtained from a traditional two-dimensional electron gas. The Landau levels observed in our transport measurements, shown in Fig. S17a,b , thus cannot arise from the quantum oscillations of a single Fermi arc state. However, the quantum Hall states in our measurements could be viewed as arising from two such Fermi arc states, which are slightly non-degenerate. In $Pt_{1-x}Au_xLuSb$ the Fermi arcs do indeed appear in pairs, which are related to each other by a 180° rotation, as shown in Fig. S17c. This rotational symmetry is maintained both at the bulk and the surface of the crystal lattice and hence, the Landau levels from such pairs of Fermi arc states are necessarily degenerate, which remains unaffected by the application of magnetic field due to their chiral nature. Therefore, we can conclusively rule out the possibility that the quantum Hall states observed in our transport measurements arises from the chiral Landau levels of Fermi arc states.

[1] Patel, S. J., et al. Surface and electronic structure of epitaxial PtLuSb (001) thin film. *Appl. Phys. Lett.* **104**, 201603 (2014).

[2] Logan, J. A., et al. Observation of a topologically non-trivial surface state in half-Heusler PtLuSb (001) thin films. *Nat. Commun.* **7**, 1-7 (2016).
[3] Seibel, E. M., et al. Gold-gold bonding: the key to stabilizing the 19-electron ternary phases LnAuSb (Ln= La - Nd and Sm) *J. Am. Chem. Soc.* **137**, 1282-1289 (2015).
[4] Strohbeen, P. J., Electronically enhanced layer buckling and Au-Au dimerization in epitaxial LaAuSb films. *Phys. Rev. Mater.* **3**, 024201 (2019).
[5] Hikami, S., Larkin, A. I., Nagaoka, Y., Spin-orbit interaction and magnetoresistance in the two dimensional random system. *Prog. Theor. Phys.* **63**, 707-710 (1980).
[6] Ando, Y., Topological insulator materials *J. Phys. Soc. Jpn.* **82**, 102001 (2003).
[7] Altshuler, B. L., Aronov, A. G., Khmelnitsky, D. E., Effects of electron-electron collisions with small energy transfers on quantum localisation. *J. Phys. C* **15**, 7367 (1982).
[8] Liao, J. et al., Enhanced electron dephasing in three-dimensional topological insulators. *Nat. Commun.* **8**, 16071 (2017).
[9] Dresselhaus, G., Spin-orbit coupling effects in zinc blende structures. *Phys. Rev.* **100**, 580 (1955).
[10] Brydon, P. M. R., Wang, L., Weinert, M., Agterberg, D. F., Pairing of j= 3/2 fermions in half-Heusler superconductors. *Phys. Rev. Lett.* **116**, 177001 (2016).
[11] Cano, J., et al. Chiral anomaly factory: Creating Weyl fermions with a magnetic field. *Phys. Rev. B* **95**, 161306 (2017).
[12] Potter, A. C., Kimchi, I., Vishwanath, A., et al. Quantum oscillations from surface Fermi arcs in Weyl and Dirac semimetals. *Nat. Commun.* **5**, 1-6 (2014).

Table S1: Band bending in $Pt_{1-x}Au_xLuSb$

| Compound | $\Delta_1$ (meV) | $\Delta_2$ (meV) | $\Delta_3$ (meV) | $\Delta_{bb}$ (meV) |
|---|---|---|---|---|
| PtLuSb | -350 | 59 | 294 | 3 |
| $Pt_{7/8}Au_{1/8}LuSb$ | 1 | 102 | 122 | 225 |
| $Pt_{5/8}Au_{3/8}LuSb$ | 2 | 149 | -28 | 123 |

Table S2: Model parameters

| Parameters | $Pt_{3/4}Au_{1/4}LuSb$ | $Pt_{1/2}Au_{1/2}LuSb$ |
|---|---|---|
| $\mu$ (meV) | 130 | 115 |
| $g$ | 6.6 | 9.4 |
| $\Delta_h$ (meV) | 73 | 48 |
| $\Delta_i$ (meV) | 3 | 3 |
| $k_F$ (Å$^{-1}$) | 0.034 | 0.033 |

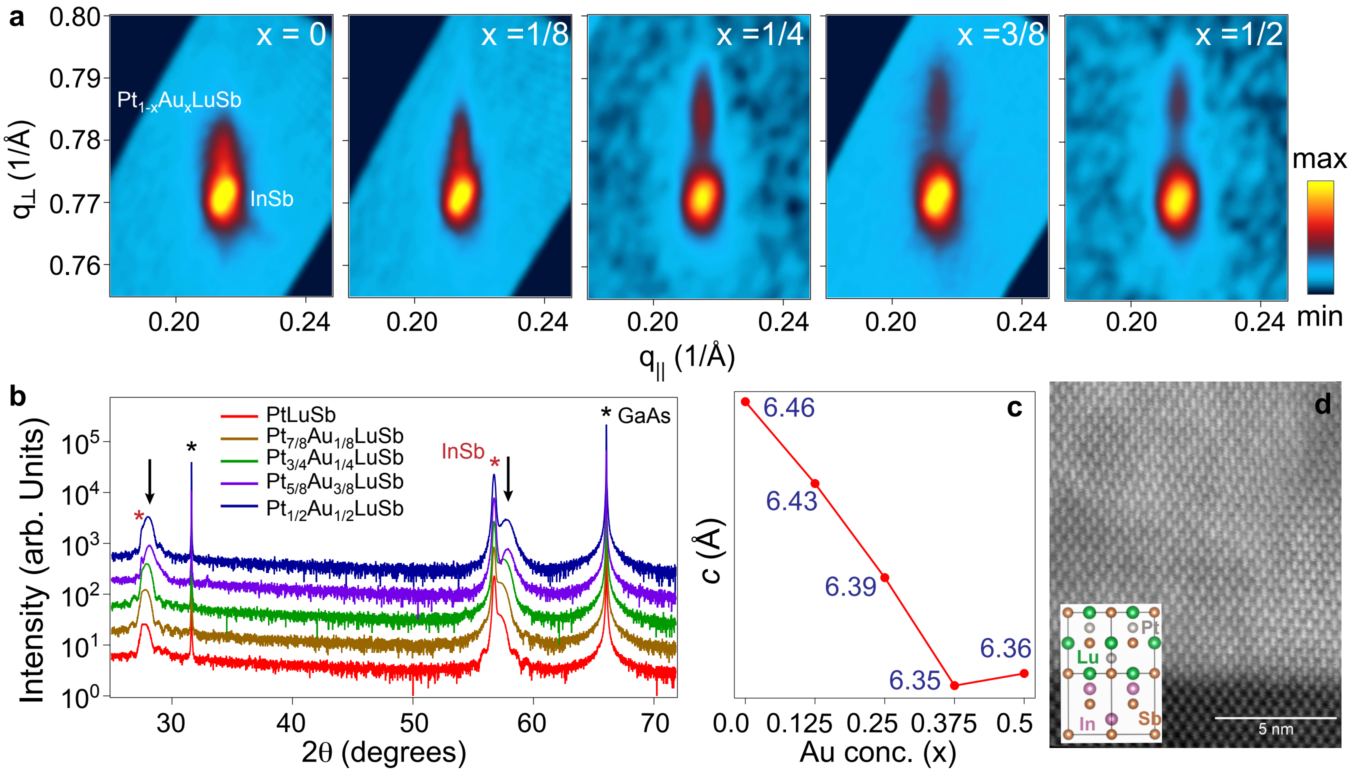


Figure S1: **Epitaxial growth and characterisation of $Pt_{1-x}Au_xLuSb$ thin films. a.** Reciprocal space maps (RSMs) of $Pt_{1-x}Au_xLuSb$ thin films for different Au concentrations showing $Pt_{1-x}Au_xLuSb$ remain pseudomorphic to the InSb buffer layer for all measured Au concentrations. Au concentrations are noted on the top-right corner of each panel. **b.** Out-of-plane $\theta$-$2\theta$ scans of $Pt_{1-x}Au_xLuSb$ thin films with different Au concentrations. Film peaks are shown with black arrows and substrate (GaAs) and the buffer (InSb) peaks are shown by black and red asterisks, respectively. **c.** Evolution of the out-of-plane lattice constant ($c$) with Au concentration. **d.** HAADF-STEM image of a 15 nm thick $Pt_{7/8}Au_{1/8}LuSb$ thin film along the [110] zone-axis. Inset shows schematic of a proposed atomic arrangement across the InSb-$Pt_{1-x}Au_xLuSb$ interface when viewed along the [110] direction.

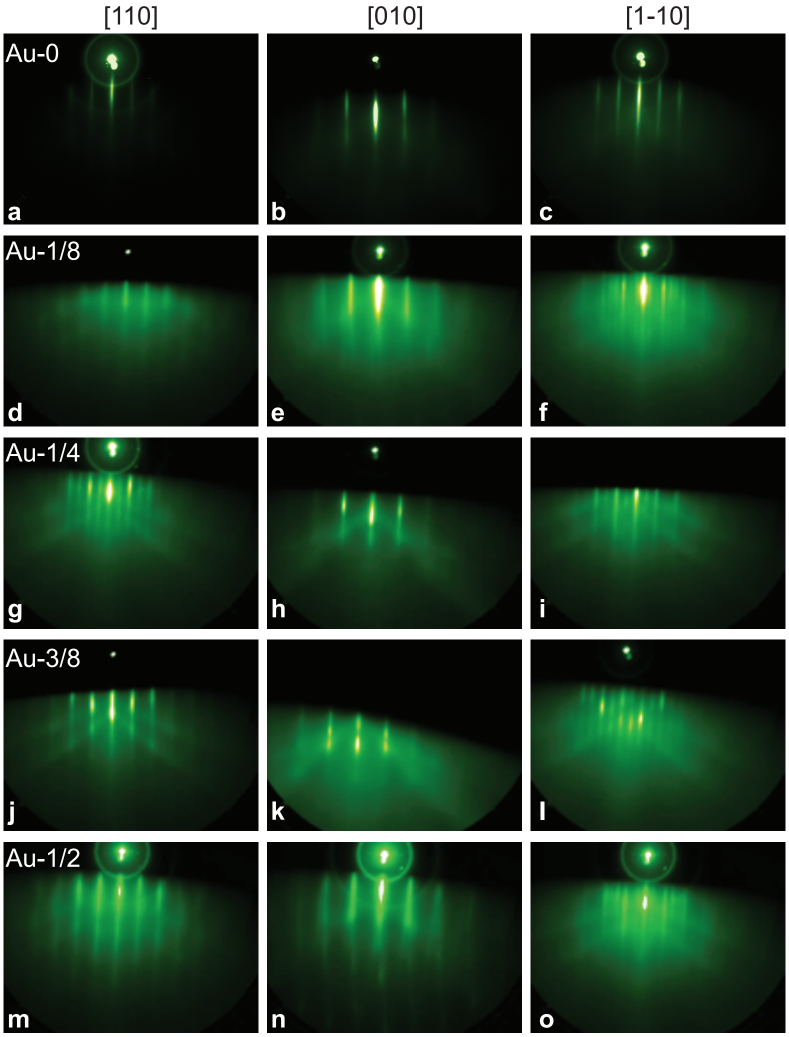


Figure S2: **RHEED images of $Pt_{1-x}Au_xLuSb$ thin films.** Reflection high-energy electron diffraction images of $Pt_{1-x}Au_xLuSb$ thin films along [110], [010], and [1-10] azimuths for **a-c.** x=0 **d-f.** x=1/8 **g-i.** x=1/4 **j-l.** x=3/8 **m-o.** x=1/2, respectively.

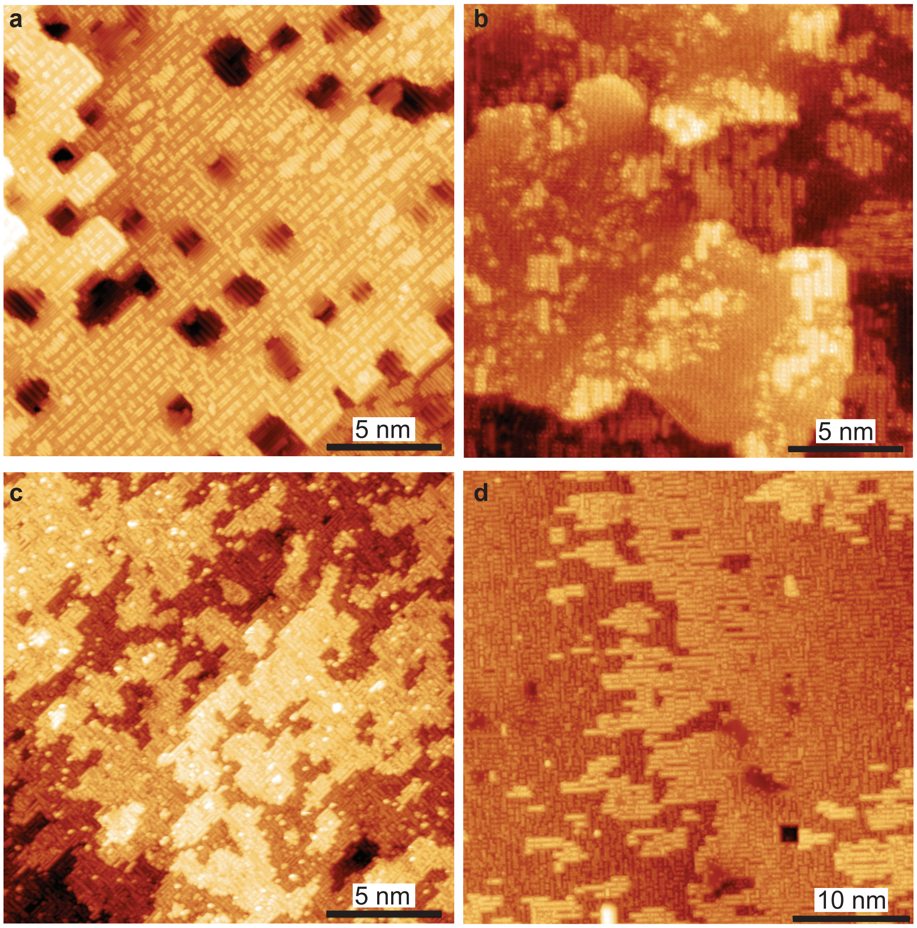


Figure S3: **Scanning tunnelling microscopy (STM) of $Pt_{1-x}Au_xLuSb$ thin films.** STM images of $Pt_{1-x}Au_xLuSb$ thin films taken at 4K sample temperature for **a.** x=0 **b.** x=1/8 **c.** 1/4 **d.** 3/8

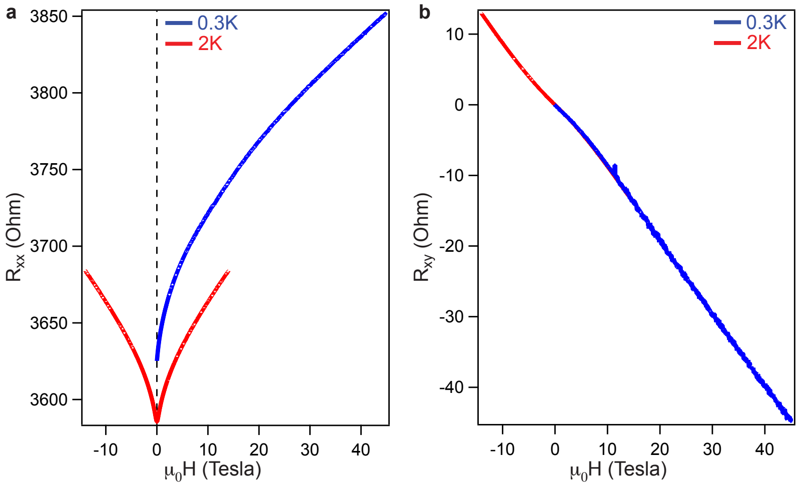


Figure S4: **Transport properties of InSb buffer layer. a.** Longitudinal and **b.** Hall resistance of the 270 nm thick InSb buffer layer on unintentionally doped GaAs substrate used to synthesize $Pt_{1-x}Au_xLuSb$ thin films.

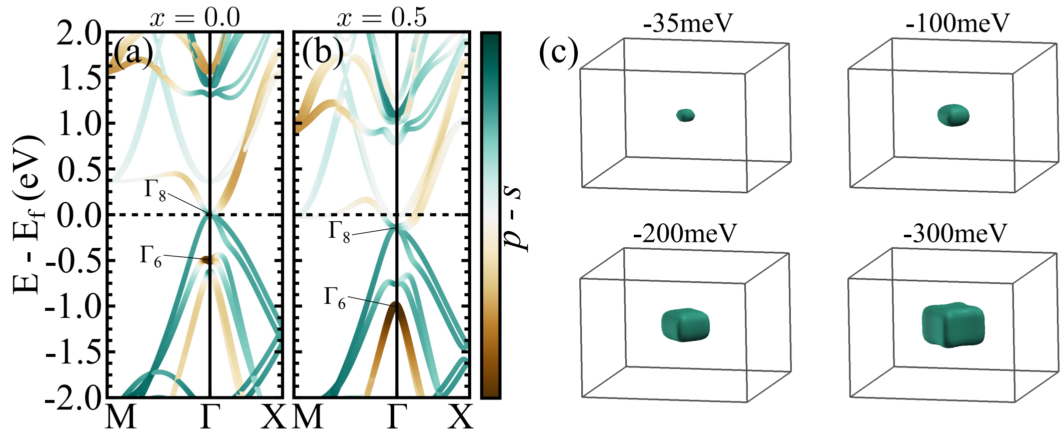


Figure S5: DFT calculation of the $s$ and $p$ character of the spin-orbit coupled bulk bands close to the Fermi energy for $Pt_{1-x}Au_xLuSb$ with (a) x = 0.0 and (b) x = 0.5. Blue (brown) color indicate the $p$ ($s$) character of each band. (c) Three-dimensional Fermi surface plots for the x=0.0 case and Fermi energy at -35 meV, -100 meV, -200 meV, and -300 meV below the $\Gamma_8$ point.

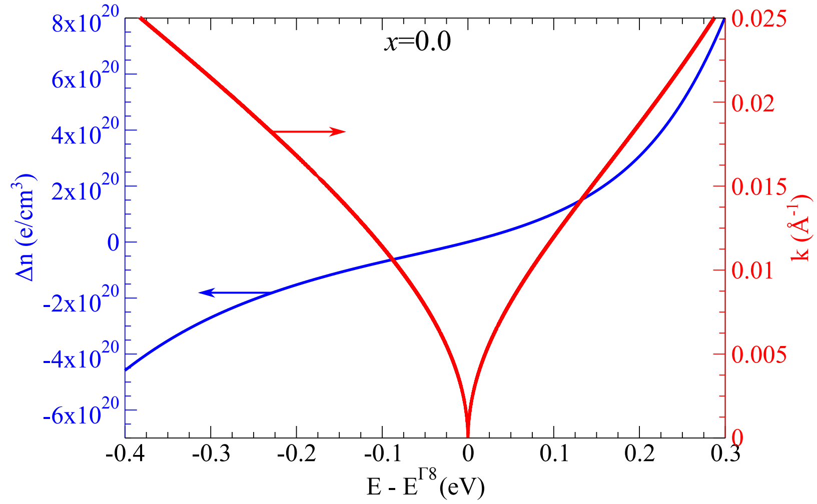


Figure S6: Evolution of the bulk carrier concentration and Fermi wavevector ($k_F$) along $\Gamma - M$ as a function of the position of the chemical potential with respect to the $\Gamma_8$ point, estimated from a bulk DFT calculation of PtLuSb.

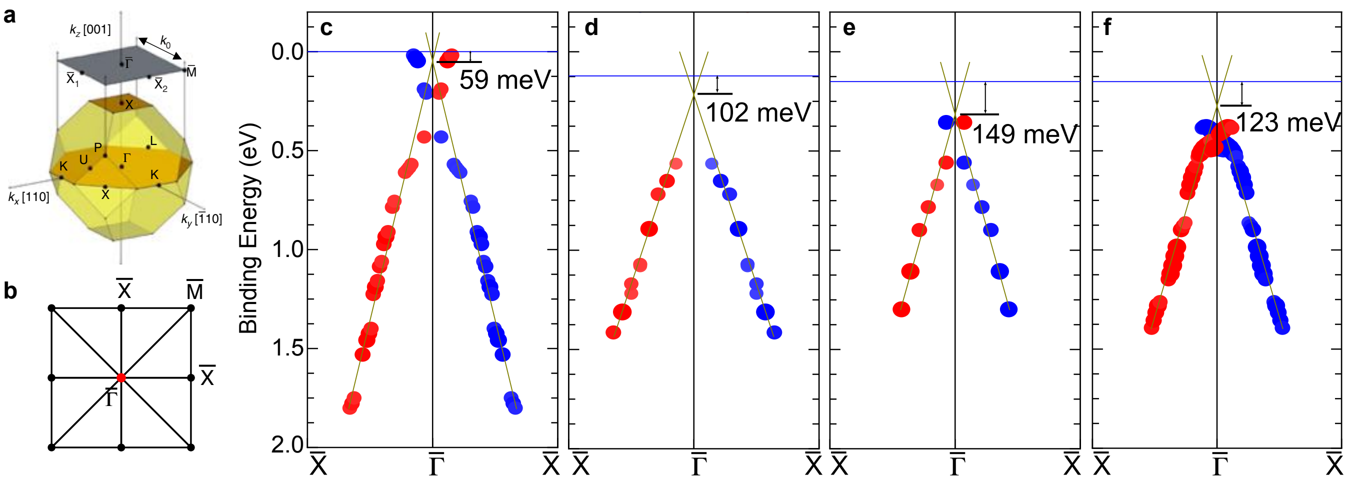


Figure S7: **Estimation of $\Delta_2$ a.** Three-dimensional (3-D) and **b.** Two-dimensional (2-D) surface Brillouin zone of $Pt_{1-x}Au_xLuSb$ showing the high symmetry points. Dispersion of the calculated topological surface state (TSS) from the slab calculations for **c.** x=0 **d.** x=1/8 **e.** x=3/8 **f.** x=1/2. Linear extrapolated crossing points (LECP) along with estimated $\Delta_2$ values are shown in corresponding panels. Binding energy of the bulk $\Gamma_8$ point is shown by blue lines. Linear fits to the dispersion of the TSS at higher binding energies is used to calculate LECP, as described in the text.

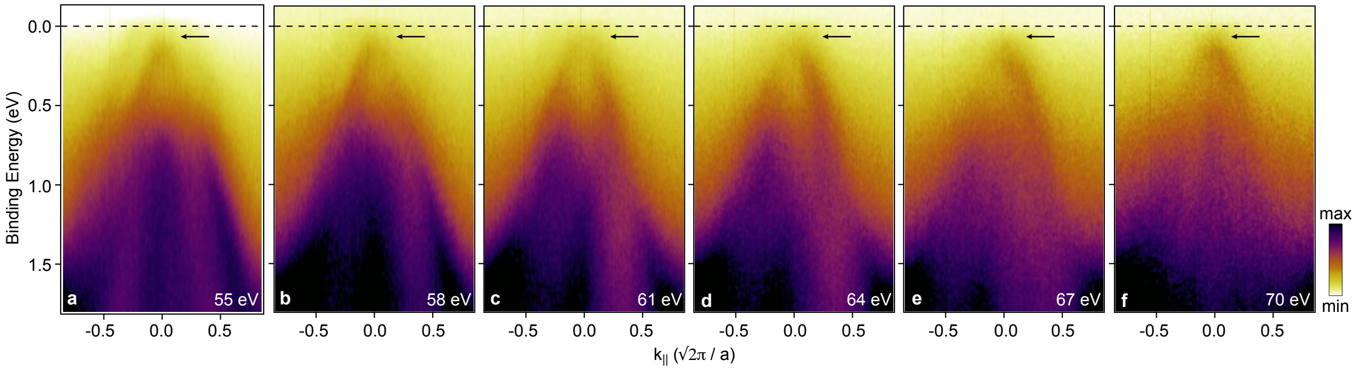


Figure S8: **Two-dimensional nature of the topological surface state (TSS) in $Pt_{1-x}Au_xLuSb$** ARPES measurements of $Pt_{5/8}Au_{3/8}LuSb$ sample at photon energies **a.** 55 eV **b.** 58 eV **c.** 61 eV **d.** 64 eV **e.** 67 eV **f.** 70 eV showing lack of dispersion in the out-of-plane direction establishing the two-dimensional nature expected from a TSS.

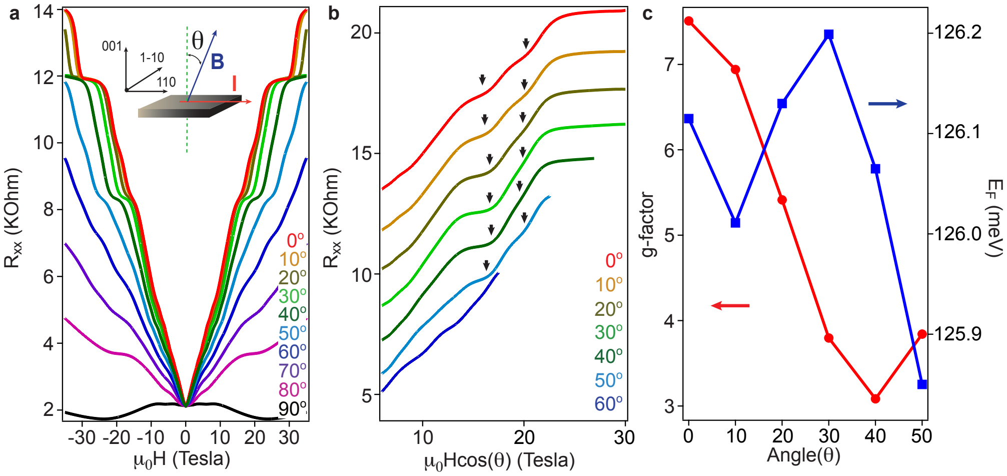


Figure S9: **Angle dependent magnetoresistance of $Pt_{7/8}Au_{1/8}LuSb$ thin films. a.** Longitudinal magnetoresistance at different tilt angle. The tilt angle between the surface normal and the magnetic field vector is shown in the inset. **b.** Same data plotted as a function of the perpendicular component of the magnetic field vector. **c** Extracted effective g-factor and Fermi level ($E_F$) from a fit to the data in **b.** (see text).

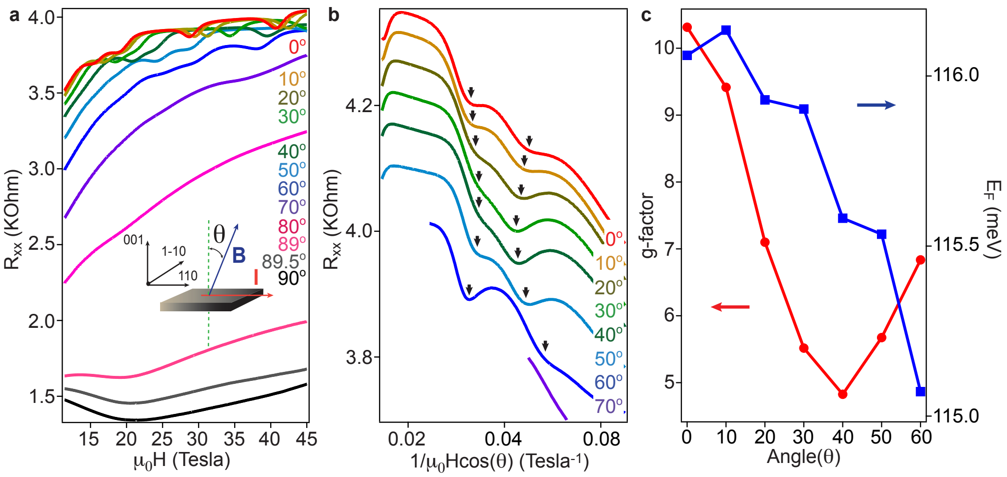


Figure S10: **Angle dependent magnetoresistance of $Pt_{5/8}Au_{3/8}LuSb$ thin films. a.** Longitudinal magnetoresistance at different tilt angle. The tilt angle between the surface normal and the magnetic field vector is shown in the inset. **b.** Same data plotted as a function of the inverse of the perpendicular component of the magnetic field vector. **c** Extracted effective g-factor and Fermi level ($E_F$) from a fit to the data in **b.** (see text).

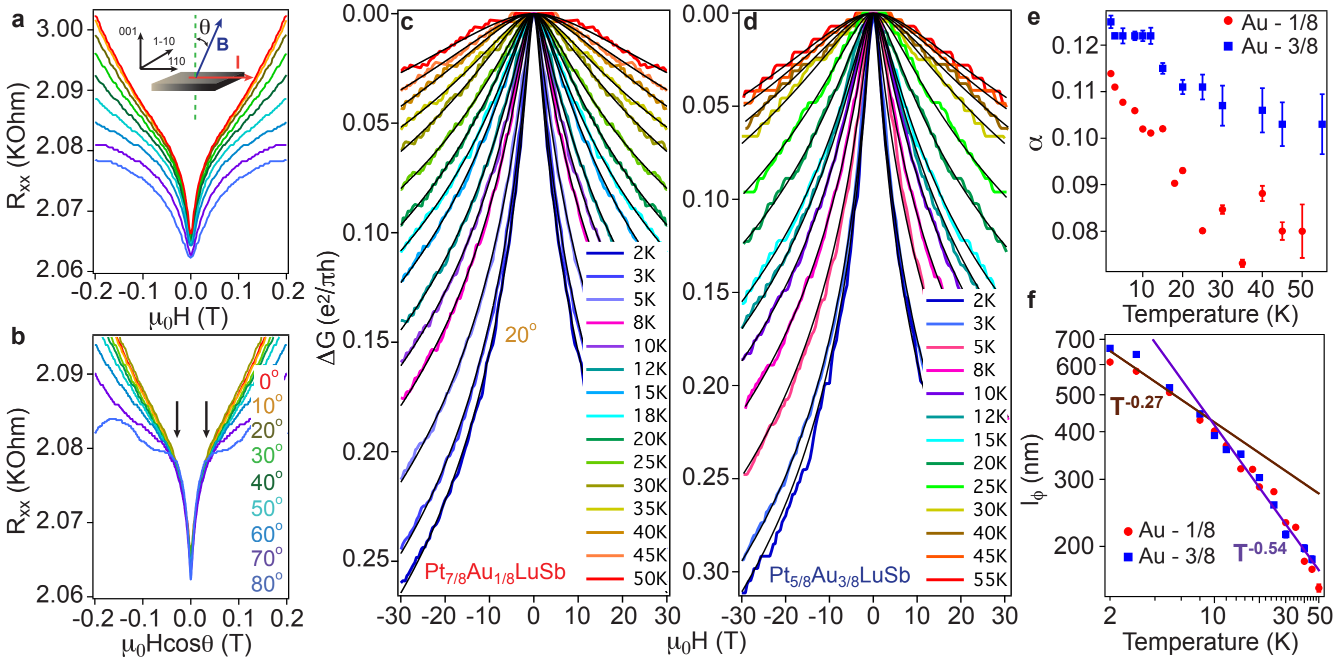


Figure S11: **Weak anti-localization in $Pt_xAu_{1-x}LuSb$ thin films a.** Weak-antilocalization (WAL) in $Pt_{7/8}Au_{1/8}LuSb$ at different tilt angles. The tilt angle between the surface normal and the magnetic field vector is shown in the inset. **b.** Same data in **a.**, but plotted as a function of the perpendicular component of the magnetic field vector. WAL behavior at low magnetic fields (the range shown by the black arrows) scales with the perpendicular component of the magnetic field vector indicating its two-dimensional character. **c-d.** Differential conductance $\Delta G(B = \mu_0 H) = G(B) - G(0)$ as a function of magnetic field and corresponding HLN fits for **c.** $Pt_{7/8}Au_{1/8}LuSb$ and **d.** $Pt_{5/8}Au_{3/8}LuSb$. Temperature dependence of the extracted **e.** pre-factor ($\alpha$) and **f.** phase coherence length ($l_\phi$) as a function of temperature.

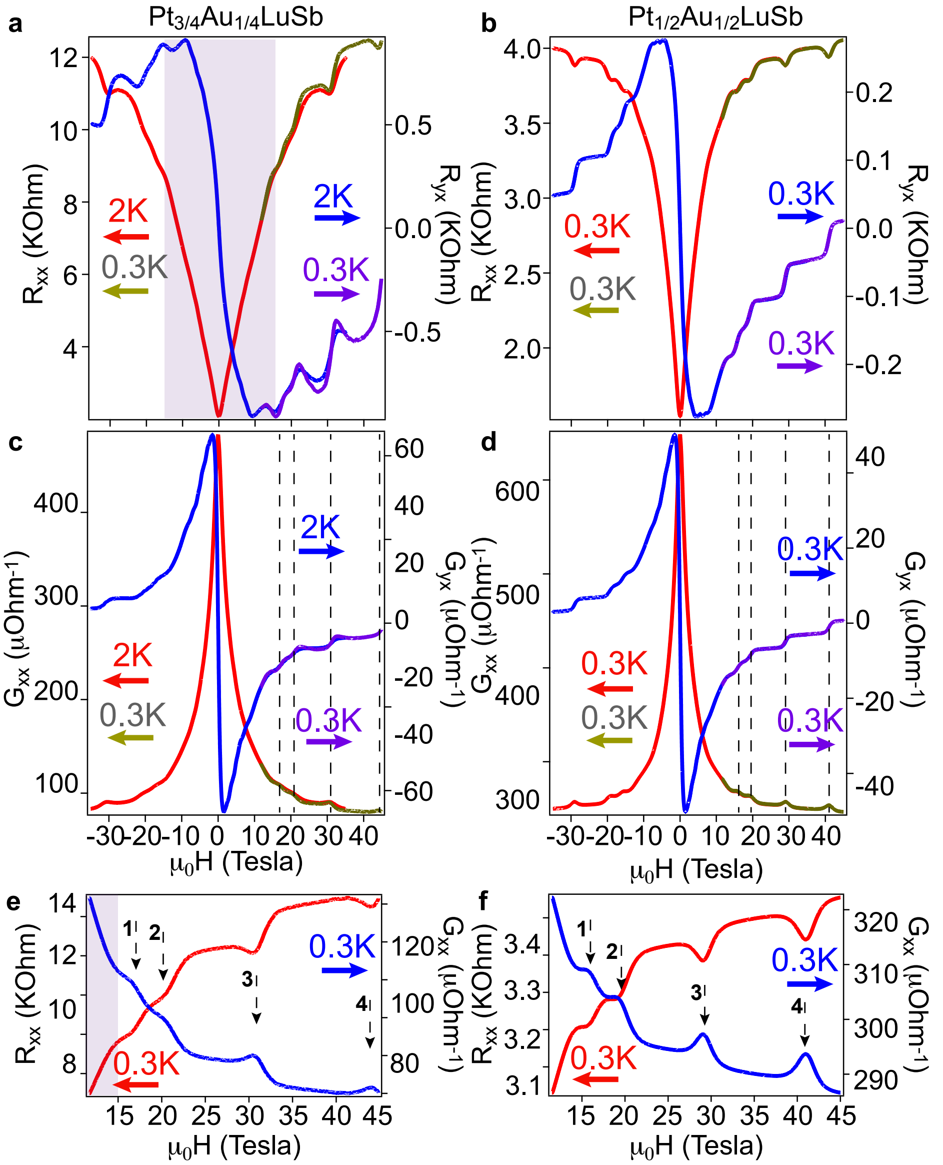


Figure S12: **Transport properties of $\mathbf{Pt_{3/4}Au_{1/4}LuSb}$ and $\mathbf{Pt_{1/2}Au_{1/2}LuSb}$.** Longitudinal and Hall resistance in **a.** $Pt_{3/4}Au_{1/4}LuSb$ and **b.** $Pt_{1/2}Au_{1/2}LuSb$. Longitudinal and Hall conductance in **c.** $Pt_{3/4}Au_{1/4}LuSb$ and **d.** $Pt_{1/2}Au_{1/2}LuSb$. Correspondence between local minima in longitudinal resistance and local maxima in longitudinal conductance in **e.** $Pt_{3/4}Au_{1/4}LuSb$ and **f.** $Pt_{1/2}Au_{1/2}LuSb$. Linear magnetoresistance behavior in $Pt_{3/4}Au_{1/4}LuSb$ is highlighted in violet in **a** and **e**. Sample temperature at which the data is taken is noted in the corresponding panels.

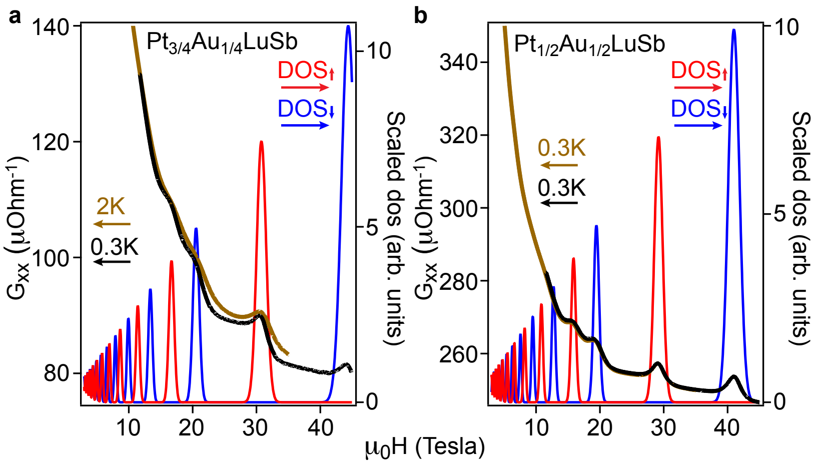


Figure S13: **Fits to the quantum Hall data in $\mathbf{Pt_{1-x}Au_xLuSb}$** Conductivity and corresponding fits to the *two-Dirac model*, as described in the text, for **a.** $Pt_{3/4}Au_{1/4}LuSb$ and **b.** $Pt_{1/2}Au_{1/2}LuSb$. $DOS_\uparrow$ and $DOS_\downarrow$ are the contributions from the Zeeman split Landau levels with spin direction along and opposite to the applied magnetic field, respectively.

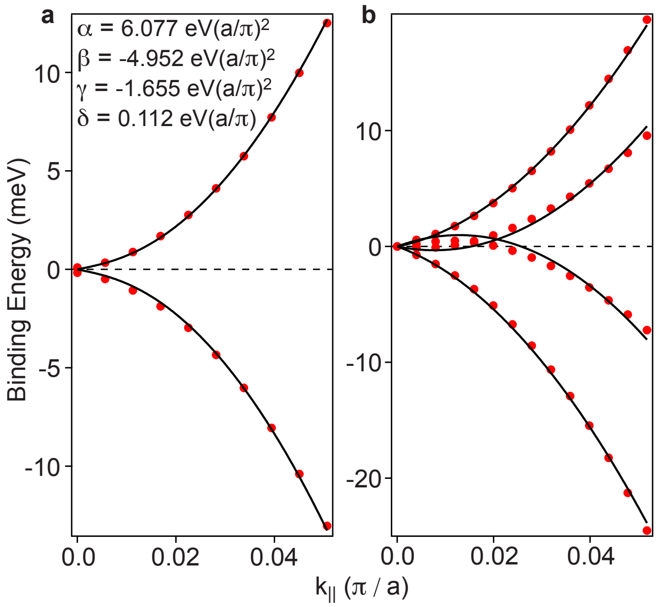


Figure S14: ***k.p* fits.** Fits to a *k.p* model as described in the text to the calculated band structure of PtLuSb from density functional theory along **a.** [100] and **b.** [110] crystallographic directions.

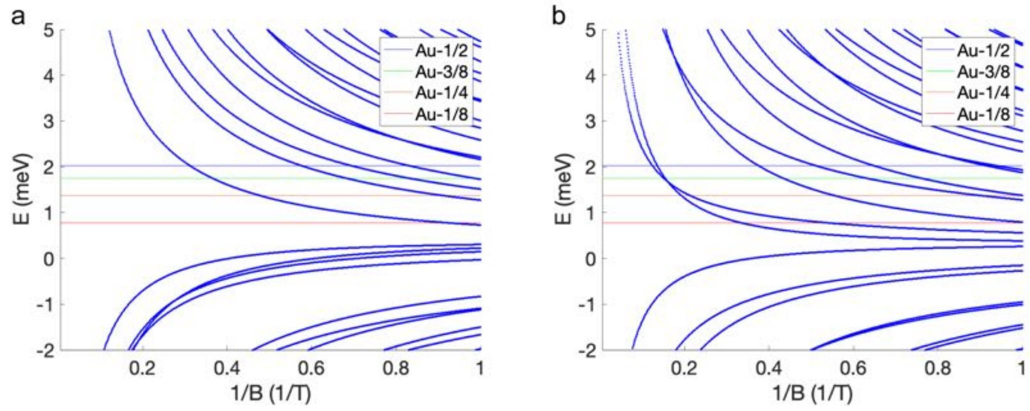


Figure S15: Landau levels $E$ vs $1/B$ for the bulk $k.p$ model (S3) with the parameters from Fig. S14, where **a.** $g = 10$ and **b.** $g = 0$ in the unit of Bohr magneton. The Fermi level at Au doping $x = 1/2$, 3/8, 1/4, and 1/8 is 2.025, 1.75, 1.375, and 0.775 meV respectively, as indicated by the blue, green, orange and pink horizontal lines, respectively. The crossings between the Landau levels and Fermi energies correspond to the edges of the Hall conductance plateaus.

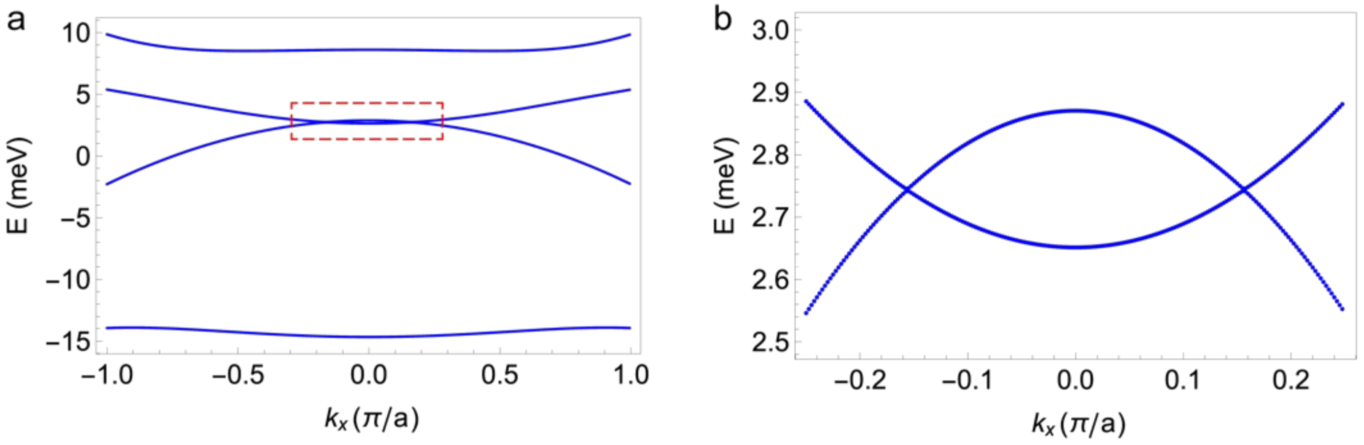


Figure S16: Weyl points arise from the protected crossings of the $J_z = 3/2$ and $J_z = -1/2$ bands when magnetic field vector $\mathbf{B}$ is added in the [001] direction. For the $k.p$ model with parameters from Fig. S14, $g = 10\ \mu_B$ and $B = 10\ T$, there are eight such crossings at $(\pm k_0, 0, \pm k_{z0})$, $(0, \pm k_0, \pm k_{z0})$, where $k_0 = 0.157$, $k_{z0} = 1.084\ \pi/a$. **a.** $E\ vs\ k_x$ at $k_y = 0\ k_z = k_{z0}$. The zoom in plot of the red dashed square in **a** is shown in **b**. The other two crossings between $J_z = 3/2$ and $J_z = 1/2$ bands are at $(0, 0, \pm 0.737\ \pi/a)$, not shown in these plots. These Weyl points project to the same point on the (001) surface, hence do not result in a non-zero Fermi arc length.

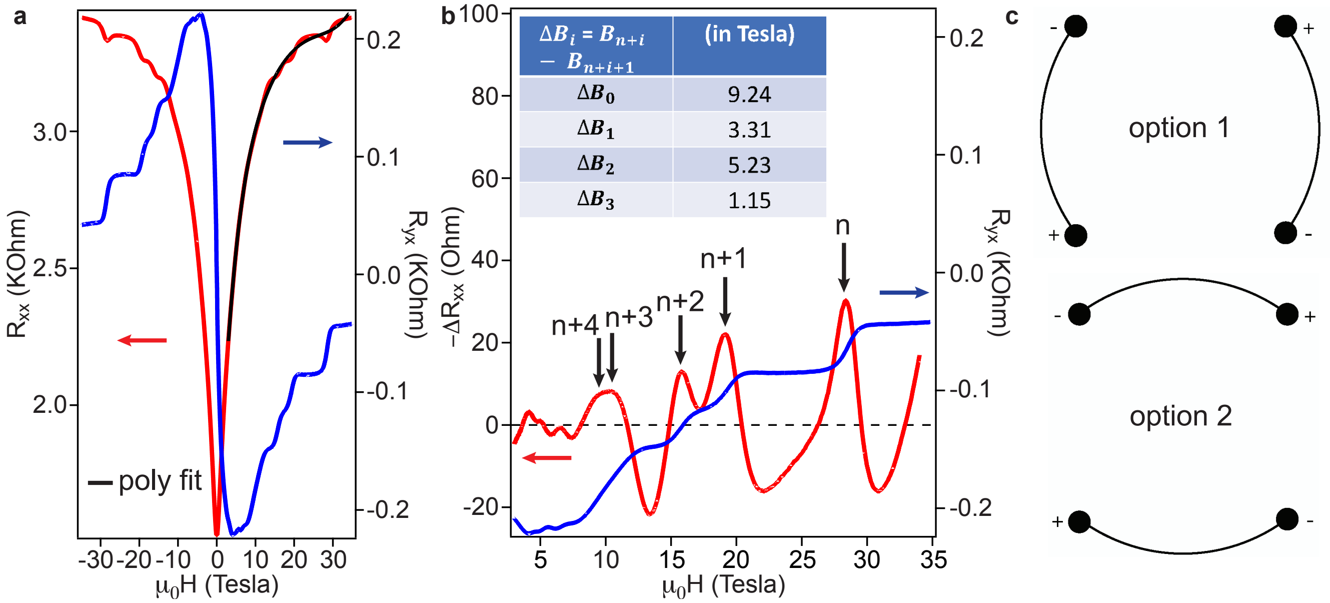


Figure S17: **Quantum oscillations and possible Fermi Arcs in $Pt_{1-x}Au_xLuSb$ a** Longitudinal magnetoresistance and Hall resistance in $Pt_{5/8}Au_{3/8}LuSb$. **b.** Resistance minima due to the Landau level crossings obtained after subtracting a smooth $7^{th}$ order polynomial (black line in **a**) from the magnetoresistance data shown in **a.**. The separation between the adjacent Landau level crossings is non-monotonic in magnetic field in contrast to the expectation from a Fermi arc state, as described in the text. **c.** Two possible pairs of Fermi arc states on the (001) surface that can arise from two pairs of Weyl points. For each such pair, the Fermi arcs are related by a 180° rotational symmetry and hence, lead to doubly degenerate Landau levels, where the degeneracy remains unaffected by the application of magnetic field due to their chiral nature.
